# Supplementary material for: A Minimal Model of the Hydrodynamical Coupling of Flagella on a Spherical Body with application to Volvox
Source: arXiv:2004.05262 ancillary file (2020-04-11)
Supplement: Supplementary file 1 [file Volvox_Supplementary_Material.pdf]

# A Minimal Model of the Hydrodynamical Coupling of Flagella on a Spherical Body: Supplementary Material

Forest O. Mannan*
*Mathematics & Computer Science Department, Western Colorado University*

Miika Jarvela and Karin Leiderman†
*Department of Applied Mathematics and Statistics, Colorado School of Mines*

## I. SUPPLEMENTARY MATERIAL

### A. Drag on a Sphere in the Vicinity of another Sphere

In the present model the modification on the drag experienced by each spherical rotor due to the spherical *Volvox* body is neglected. Generally, the drag is decomposed into a parallel and perpendicular component between the center of the two spheres. Since the drag is greatest in the perpendicular direction and we seek only a bound on the overall drag, it suffices to consider only the perpendicular direction. Assuming the *Volvox* body remains stationary the percentage modification to the free space drag experienced by a rotor moving with velocity $\mathbf{v}$ is given by

$$\frac{9}{4}\frac{aR_v}{l^2} + \frac{3}{4}\left(-2\frac{a^3 R_v}{l^4} + \frac{27}{4}\frac{a^2 R_v^2}{l^4} + 3\frac{aR_v^3}{l^4}\right)$$

where $a$ is the radius of the rotor, $R_v$ is the radius of the *Volvox* and $l$ is the distance between the center of the two spheres [1]. Assuming the parameters specified in text and using the worst case $l$ corresponding to the nadir of the preferred orbit, the error is $\approx 2.7\%$ of the free space drag.

### B. Regularization Parameter Sensitivity

The sensitivity of the rotor dynamics to the choice of regularization parameter is investigated by considering the phase difference between two coupled rotors above a plane. For fixed initial phases, we varied the regularization parameter and evolved the rotors in time. As Figure 1 shows, varying the regularization parameter over two orders of magnitude has no discernible effect on the dynamics of the evolution of the phase difference of two rotors. This suggests that the simulation results are not heavily dependent on the regularization parameter used.

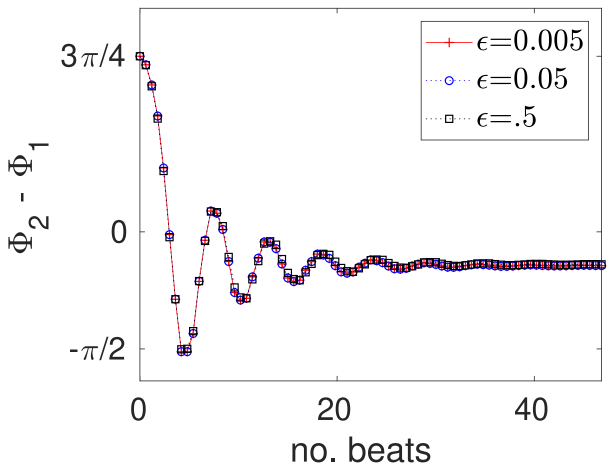


FIG. 1: The dynamics of two rotors above a plane. The range of regularization parameters considered has indistinguishable effects on the dynamics. The simulations presented in the paper correspond to $a/d = 0.1$.

### C. Idealized Rotor Schematics

Figure 2 shows a schematic of a portion of the idealized rotors around the equator and in the meridional direction. At any point in time, each idealized rotor is assigned a phase equal to the average phase of all rotors within a distance of $2.5d$, as described in the paper. To illustrate this, the rotors within $2.5d$ of the tenth idealized rotor around the equator and along a meridian are shown in blue.

### D. Comparing the Fluid Velocities Induced by Horizontal and Diagonal Steady States

All simulations ran tended towards one of two steady states; either a horizontal metachronal wave or a diagonal metachronal wave. As Figure 3 shows, the induced velocities in the surrounding fluid, averaged over one full period, are nearly identical. Despite this, it should be noted that the induced velocities at any given snapshot are significantly different. The video HorizontalAndDiagonalSnapshots.mp4 shows the induced fluid velocities

* fmannan@western.edu
† kleiderman@mines.edu

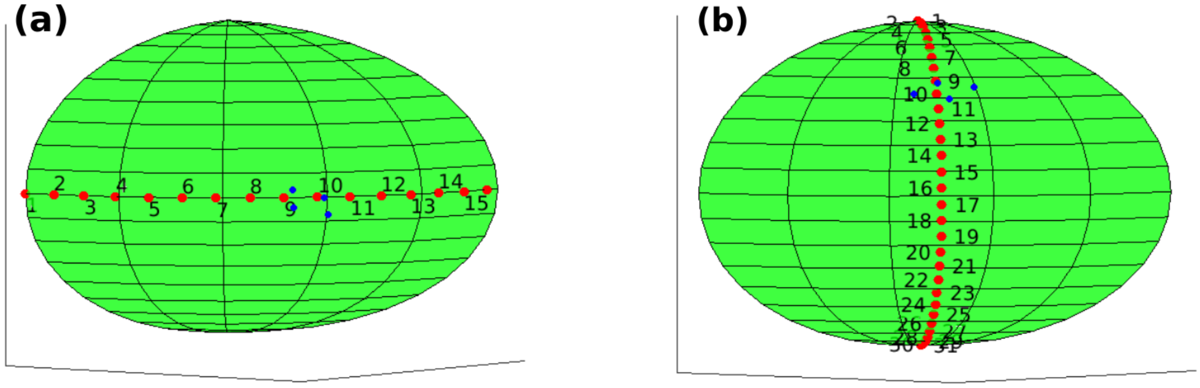


FIG. 2: A portion of the idealized rotors are shown in red and are equally spaced around the equator (a) and a meridian (b). The idealized rotors are numbered and the rotors within $2.5d$ of the tenth idealized rotor are shown in blue.

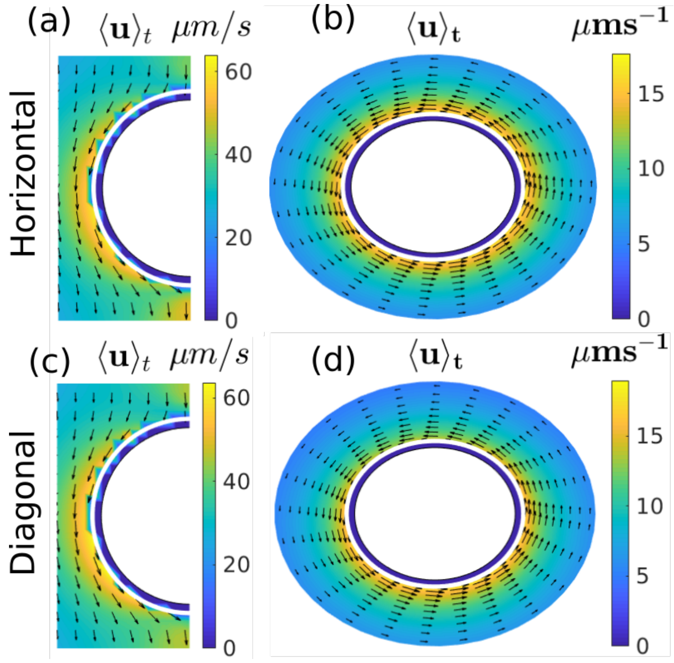


FIG. 3: (a) and (c) show the fluid velocities, averaged over one full period, in the meridional plane for a horizontal and a diagonal steady state respectively. (b) and (c) show the fluid velocities in the equatorial plane, averaged over one full period, for a horizontal and a diagonal steady state respectively.

in a full meridional plane for both steady states over 3 periods.

[1] J. Happel and H. Brenner, *Low Reynolds number hydrodynamics: with special applications to particulate media*, Vol. 1 (Springer Science & Business Media, 2012).
